# Supplementary material for: GeneOH Diffusion: Towards Generalizable Hand-Object Interaction Denoising via Denoising Diffusion
Source: arXiv:2402.14810 source file (2024-02-22)
Supplement: Supplementary file 1 [file main_wo_appendix.tex]

\documentclass{article} % For LaTeX2e
\usepackage{iclr2024_conference,times}

% Optional math commands from https://github.com/goodfeli/dlbook_notation.
\input{math_commands.tex}

\usepackage{hyperref}
\usepackage{url}

\usepackage{graphicx}
\usepackage{makecell}
\usepackage{booktabs}
\usepackage{multirow}
\usepackage{multicol}
\usepackage{algorithm}
\usepackage{algorithmicx}
\usepackage{colortbl}

\usepackage{wrapfig}

\usepackage[noend]{algpseudocode} % http://ctan.org/pkg/algorithmicx

\title{GeneOH Diffusion: Towards Generlaizable Hand-Object Interaction Denoising via Denoising Diffusion}

% Authors must not appear in the submitted version. They should be hidden
% as long as the \iclrfinalcopy macro remains commented out below.
% Non-anonymous submissions will be rejected without review.

\author{Antiquus S.~Hippocampus, Natalia Cerebro \& Amelie P. Amygdale \thanks{ Use footnote for providing further information
about author (webpage, alternative address)---\emph{not} for acknowledging
funding agencies.  Funding acknowledgements go at the end of the paper.} \\
Department of Computer Science\\
Cranberry-Lemon University\\
Pittsburgh, PA 15213, USA \\
\texttt{\{hippo,brain,jen\}@cs.cranberry-lemon.edu} \\
\And
Ji Q. Ren \& Yevgeny LeNet \\
Department of Computational Neuroscience \\
University of the Witwatersrand \\
Joburg, South Africa \\
\texttt{\{robot,net\}@wits.ac.za} \\
\AND
Coauthor \\
Affiliation \\
Address \\
\texttt{email}
}

% The \author macro works with any number of authors. There are two commands
% used to separate the names and addresses of multiple authors: \And and \AND.
%
% Using \And between authors leaves it to \LaTeX{} to determine where to break
% the lines. Using \AND forces a linebreak at that point. So, if \LaTeX{}
% puts 3 of 4 authors names on the first line, and the last on the second
% line, try using \AND instead of \And before the third author name.

%\iclrfinalcopy % Uncomment for camera-ready version, but NOT for submission.
\begin{document}

\newcommand{\vpara}[1]{\vspace{0.07in}\noindent\textbf{#1}\xspace}
\newcommand{\todo}[1]{\textcolor{red}{todo: #1}}
\newcommand{\zz}[1]{\textcolor{mygreen}{(#1)}}
\newcommand{\summary}[1]{\textcolor{mypurple}{(#1)}}
\newcommand{\subsummary}[1]{\textcolor{myclassicblue}{[#1]}}
% ConstDiff
% CasDiff
% ChoiDiff
% \newcommand{\model}[0]{ChoiDiff~}
% \newcommand{\model}[0]{CasDiff~}
\newcommand{\model}[0]{Ours~}
% \newcommand{\rep}[0]{ConSTeRM~}
% CONSIsT
% ConsTRealm
% CasDiff
% \newcommand{\rep}[0]{CONSIsT~}
% \newcommand{\rep}[0]{CONSIST~}
% GeneOH
\newcommand{\rep}[0]{GeneOH~}
\newcommand{\repns}[0]{GeneOH}
\newcommand{\nnarticat}[0]{3~}
\newcommand{\nnrigidcat}[0]{6~}
\newcommand{\nntestsets}[0]{4~}

\maketitle

% \begin{abstract}
% The abstract paragraph should be indented 1/2~inch (3~picas) on both left and
% right-hand margins. Use 10~point type, with a vertical spacing of 11~points.
% The word \textsc{Abstract} must be centered, in small caps, and in point size 12. Two
% line spaces precede the abstract. The abstract must be limited to one
% paragraph.
% \end{abstract}

\input{articles/abstract}
\input{articles/intro}
\input{articles/related}
\input{articles/method}
\input{articles/exp}
\input{articles/aplications}
\input{articles/ablations}
% \section{}

% \appendix

% \input{supp/method}
% \input{supp/exp}

\bibliography{ref}
\bibliographystyle{iclr2024_conference}

\end{document}
