# Supplementary material for: GeneOH Diffusion: Towards Generalizable Hand-Object Interaction Denoising via Denoising Diffusion
Source: arXiv:2402.14810 source file (2024-02-22)
Supplement: Supplementary file 2 [file conclusions.tex]

% \section{}
